# Supplementary material for: Flavor structure of generalized parton distributions from neutrino experiments
Source: arXiv:1210.4825 ancillary file (2012-12-29)
Supplement: Supplementary file 1 [file README.pdf]

## Code for evaluation of $\nu$ DVMP cross-sections

This package provides a library `libDVMP` which may be used for evaluation of the  $\nu$ DVMP cross-sections with various GPD models. Below are given short instructions how to compile and use it.

**Description:** This package provides a library `libDVMP` which may be used for evaluation of the  $\nu$ DVMP cross-sections in the framework discussed in the paper. To evaluate the differential cross-section in your code, You should call function

```
double dvmp_XSection_dlnx_dt_dQ2(AbstractGPD
    fun, double* kins, process p);
```

which evaluates unintegrated cross-section  $x_B d^3\sigma/dt dx_B dQ^2 = \nu d^3\sigma/dt d\nu dQ^2$ , or

```
double dvmp_XSection_dlnx_dQ2(AbstractGPD
    fun, double* kins, process p);
```

which evaluates the  $t$ -integrated cross-section  $x_B d^2\sigma/dx_B dQ^2 = \nu d^2\sigma/d\nu dQ^2$ .

Both functions are declared in `headers/DVMP_XSection.h`. The first argument `fun` corresponds to a GPD function declared in `headers/GPDPDF.h`, the array `kins` contains kinematic variables ordered as<sup>1</sup> `kins[] = {y, x_B, t, Q}`, where  $y = p \cdot q / p \cdot k$ ,  $x_B$  is a Bjorken variable,  $t$  is the momentum transfer squared,  $t = \Delta^2$ ,  $Q = \sqrt{-q^2}$ .

The structure `process p` declared in `headers/phys.h` contains information on particles participating in the process and has the following elements:

|                            |                                                                                        |
|----------------------------|----------------------------------------------------------------------------------------|
| <code>p.projectile</code>  | initial lepton ( $\nu/\bar{\nu}$ )                                                     |
| <code>p.target</code>      | target ( $p/n$ )                                                                       |
| <code>p.finalMeson</code>  | produced meson from octet of pseudogolstones ( $\pi^{0,\pm}, K^{L,S}, K^{\pm}, \eta$ ) |
| <code>p.finalBaryon</code> | produced baryon from lowest octet ( $p, n, \Lambda, \Sigma^{0,\pm}$ )                  |
| <code>p.finalLepton</code> | produced lepton ( $\nu, \bar{\nu}, \mu^{\pm}$ )                                        |

The GPD models needed for numerical evaluations are placed in separate library files in folder `libraries/`. With this package, we provide the Kroll-Goloskokov [1, 2] GPD model (file `libKrollGoloskokovGPD.so`) and a simple zero skewness GPD model (`libZeroSkewness.so`) described in the text of the paper.

**Prerequisites:** To compile this code, You need to have C compiler, `make` utility and a GNU scientific library (GSL) installed. The code was tested with `gcc` v. 4.4 and 4.6 on Linux x86-64 platform.

**Compilation:** To compile the code, You have to run `make` all in the code main directory. This will build the two above-mentioned GPD libraries, the  $\nu$ DVMP library (`libDVMP.so`, `libDVMP.a`) and an example driving application `NuDVMP` (see `src/DVMP.c`) which shows how to load GPDs from corresponding libraries and evaluate the cross-section.

**Running:** After compilation, run from command-line

```
./NuDVMP --NeutrinoType NuMuBar --Target
Proton --Lepton MuPlus --Meson PiZero
--Baryon Neutron --lepton-fraction
0.5 --virtuality 2 --gpd-model
libraries/libKrollGoloskokovGPD.so
```

or in a brief form

```
./NuDVMP -N NuMuBar -T Proton -L MuPlus
-M PiZero -B Neutron -y 0.5 -q 2 -g
libraries/libKrollGoloskokovGPD.so
```

(optionally, instead of particle names, You can use their PDG codes; only particles and processes mentioned in the text of the paper are supported). This will evaluate the cross-section  $x_B d^3\sigma/dt dx_B dQ^2$  for the process  $\bar{\nu}p \rightarrow \mu^+ \pi^0 n$  as a function of  $x_B$  at virtuality  $\sqrt{Q^2} = 2$  GeV and  $y = 0.5$ , with  $\Delta_{\perp} = 0$  (hard-coded in example routine for simplicity) and using Kroll-Goloskokov GPD model.

**Adding new GPD models:** In order to add a new GPD model, You have to implement the function `ExternalGPD(double x, struct GPDKins k)`, where `x` is the quark light-cone fraction and `struct GPDKins` declared in `headers/GPDPDF.h` keeps all the information on the target kinematics and has the following elements:

|                         |                                                                                                                 |
|-------------------------|-----------------------------------------------------------------------------------------------------------------|
| <code>k.xi</code>       | skewness parameter $\xi$                                                                                        |
| <code>k.t</code>        | momentum transfer $t = \Delta^2$                                                                                |
| <code>k.Q</code>        | Scale at which GPD is taken                                                                                     |
| <code>k.flavour</code>  | GPD flavor                                                                                                      |
| <code>k.GPD_type</code> | Type of GPD, can be <code>GPD_H</code> , <code>GPD_E</code> , <code>GPD_HTilde</code> , <code>GPD_ETilde</code> |

<sup>1</sup> Parameter  $t$  is ignored in case of  $t$ -integrated cross-section.

After compilation of the file `libNewGPD.so`, You may try to generate the cross-section using `--gpd-model` option discussed above.

For more details, please see the header files in `headers/` di-

rectory. Each function has a Doxygen-style comments with detailed description. Corresponding `.c`-files are in `src/` directory.

---

[1] S. V. Goloskokov and P. Kroll, Eur. Phys. J. C **50**, 829 (2007) [hep-ph/0611290].

[2] S. V. Goloskokov and P. Kroll, Eur. Phys. J. C **53**, 367 (2008) [arXiv:0708.3569 [hep-ph]].
